# Supplementary material for: Mitigating Leakage from Data Dependent Communications in Decentralized Computing using Differential Privacy
Source: arXiv:2112.12411 source file (2021-12-23)
Supplement: Supplementary file 1 [file Appendix3.tex]

In our context, the number of secure channels between nodes must remain limited because we are considering end-user devices with limited resources. To give an idea of the maximum limit that should not be exceeded for a feasible solution, we give here as an example a simple computation considering SGX enclaves communicating with the WolfSSL library, which shows a limit to a few hundred connections per compute node. 

We give here an approximate value for the number of secure channels which can be maintained inside a given Intel SGX enclave running on a given personal computer (given hardware). We consider an Enclave Page Cache (EPC) memory region of 128 MB, as usually made available by Intel SGX on a single hardware platform and considered in the literature (see, e.g., [\rf]). Removing the space occupied by SGX dedicated structures and code including the SGX Secure Enclave Control Structure (SECS) and the Enclave Page Cache Map (EPCM), $fp=90MB$ remain for the enclave code and data structures on the memory heap, aligned on 4KB memory blocs. To estimate the maximum number of Threads Context Structure (TCS), we consider a minimum stack and a heap of $fp_1=4KB$. 

As a value for the footprint of the implementation of a secure channel, we consider the WolfSSL module (see \url{https://www.wolfssl.com/wolfssl-with-intel-sgx}), an SGX implementation of secure channels close to MbedTLS (with available information about the memory consumption, available in the documentation at \url{https://www.wolfssl.com/wolfssl-build-sizes}). According to the WolfSSL documentation, the memory footprint of the library is up to $fp_2=100KB$. 

Obviously, the memory usage at runtime for a connection as well as the size of the input/output buffers depends on the scenario and of the role of the considered node. According to the WolfSSL documentation, for 16KB buffers (correct for a throughput of about 10KB/s), the memory usage of a connection is $fp_3=35KB$. We ignore the code footprint of the computing node (e.g., for a scrambler in our context this is around 20KB) and the memory used to manage internal operator structures (e.g., $(n+d)\times r$ with $r$ the size of an encrypted record, $n$ the number of messages considered in input and $d$ the number of additional dummy records). This gives up to $647$ connections with the above estimates, i.e., $fp / (fp_1 + fp_2 + fp_3)$.
